# Supplementary material for: Ice-Templated W-Cu Composites with High Anisotropy
Source: arXiv:1708.06801 ancillary file (2017-08-22)
Supplement: Supplementary file 1 [file Supplementary_Information.pdf]

# Supplementary Information for:
# Ice-Templated W-Cu Composites with High Anisotropy

André Röthlisberger[1,2†♮], Sandra Häberli[1∠], Henning Galinski[1†], David C. Dunand [3] & Ralph Spolenak[1]

[1]*Laboratory for Nanometallurgy, Department of Materials, ETH Zurich, Vladimir-Prelog-Weg 1-5/10, CH-8093 Zürich, Switzerland*

[2]*Mechanical Integrity of Energy Systems, Swiss Federal Laboratories for Materials Science and Technology, EMPA, CH-8600 Dübendorf, Switzerland*

[3]*Department of Materials Science and Engineering, Northwestern University, Evanston, IL 60208, USA*

† These authors contributed equally to this work

♮ currently at BIOTRONIK, Switzerland

∠ currently at ABB, Switzerland

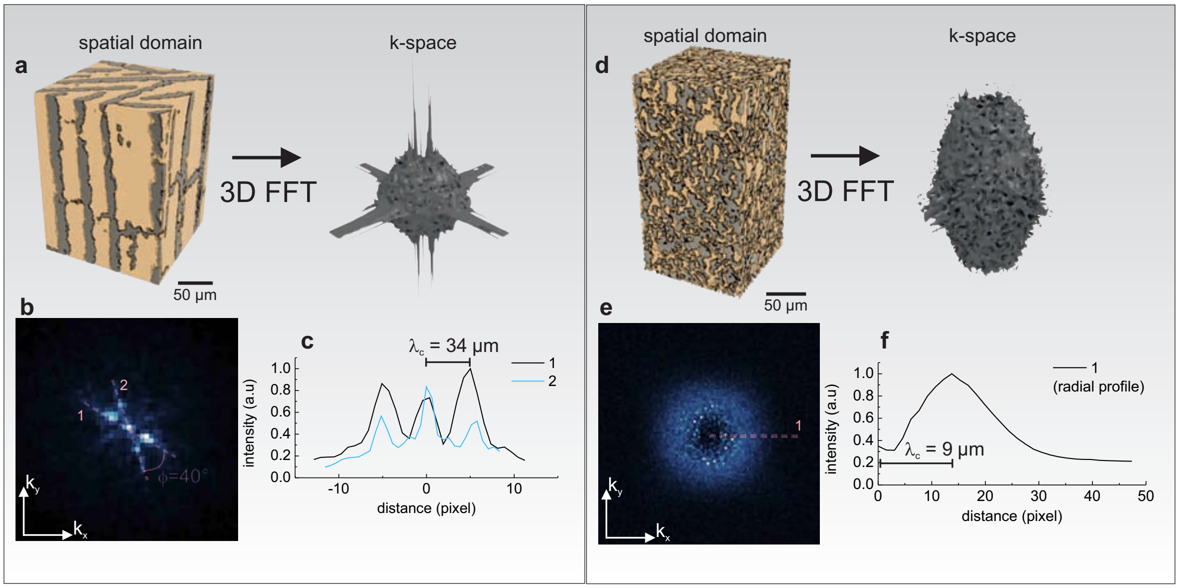


**Figure S1 – FFT Analysis.** (a) Three-dimensional Fast Fourier transformation (FFT) of the ice-templated W-Cu composite structure obtained by XCT using Parallel FFTJ and ImageJ. (b) x-y plane of the FFT, bright spots in k-space are indicating a clear spatial periodicity and structural anisotropy. Two features, i.e. two type of W-lamellae, with similar periodicity but rotated 40° relative to each other can be identified. (c) Line profiles along two directions (1,2) highlighted in (b) are shown. These profiles are used to measure the mean spatial frequency of the structure $34(2)$ $\mu$m. (d) Three-dimensional Fast Fourier transformation (FFT) of the powder-based W-Cu composite structure obtained by XCT using Parallel FFTJ and ImageJ. (e) x-y plane of the FFT, with a diffuse ring in k-space is indicating a highly isotropic structure with no distinct periodicity. (f) Line profile (1) highlighted in (e) is depicted, revealing a mean spacing between the Cu and W phases of $9$ $\mu$m.

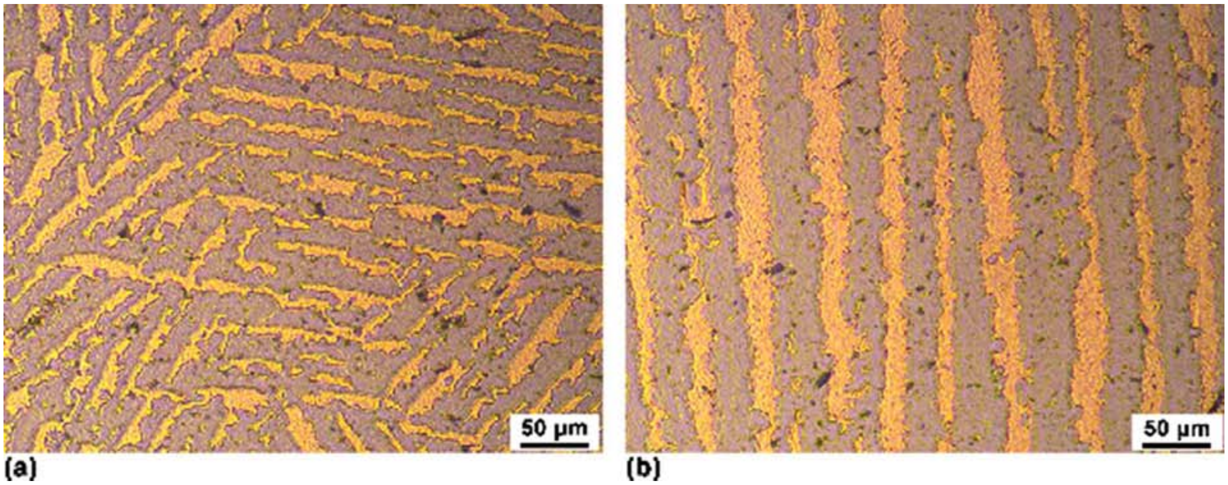


**Figure S2 – Microstructure Analysis.** Radial (a) and longitudinal (b) metallographic cross-section of a W-Cu composite (43 vol.% Cu) synthesized by freeze-casting. The architecture is clearly anisotropic with the tungsten exhibiting the typical directional structure inherent to the freeze-cast foams and the copper filling the open porosity. The orientation of the walls is random in radial direction, while along the cylinder axis (longitudinal) it is parallel. The black spots are pores from the inherent closed porosity and from the metallographic preparation.

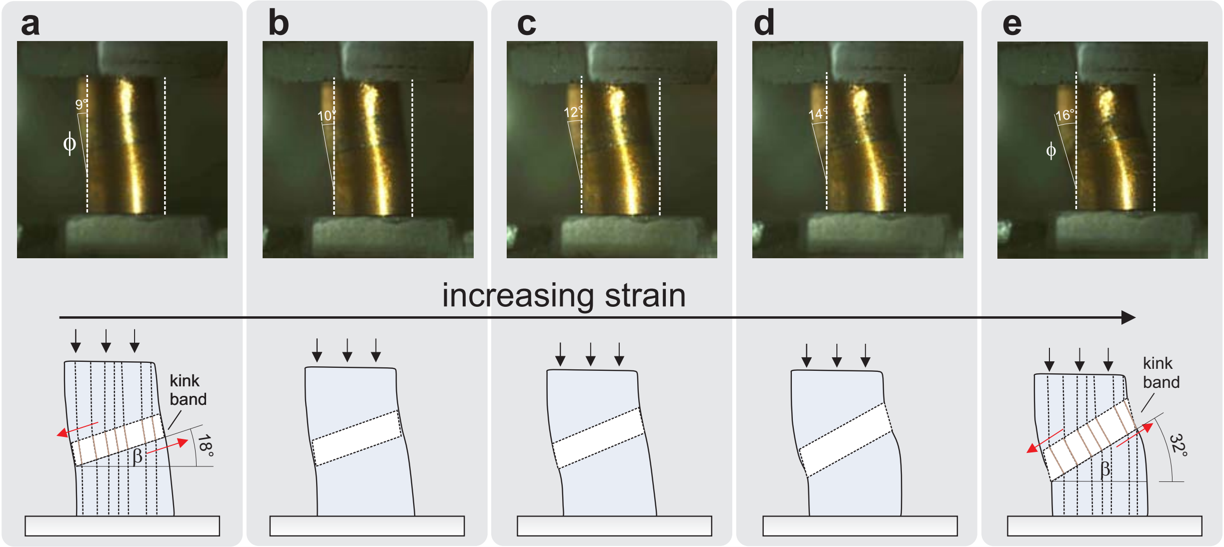


**Figure S3 – Kink band propagation.** Sequence of photographs (a)-(e) of an ice-templated W-Cu composite (43 vol.% Cu) during compressive testing illustrating kink band formation. The strain increases from left (a) to right (b). The outline of each sample is depicted together with the position and orientation of the kink band. For all states of compression, the rotation of the material, i.e. the angle of misorientation $\phi$ and the angle between the deformed and undeformed material $\beta$ hold the relationship $\phi = 2\beta$, which is characteristic for kink band formation and propagation.

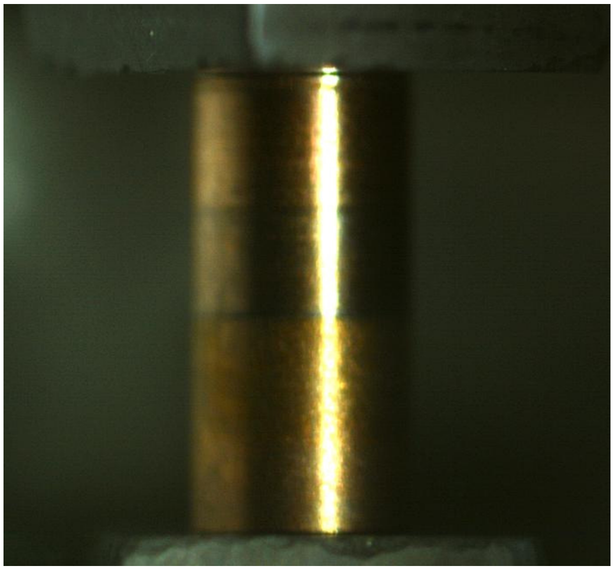

**Video S1 – Compression Test.** Video shows a compression test of an ice-templated W-Cu composite (43 vol.% Cu). During compression the sample exhibits kink band formation, i.e. a deformed and rotated band is formed within the sample.
